# Supplementary material for: Computing Augustin Information via Hybrid Geodesically Convex Optimization
Source: arXiv:2402.02731 source file (2024-05-09)
Supplement: Supplementary file 1 [file non-smoothness.tex]

\section{Proof of Proposition \ref{lemma:non-smoothness}}

For ease of notation, we adapt the notation defined in Section \ref{sec:application}.
The gradient of $f_\alpha$ is
\begin{equation*}
    \nabla f_\alpha(x)=-\mathbb{E}_p\frac{p^\alpha \odot x^{-\alpha}}{\langle p^\alpha, x^{1-\alpha}\rangle},
\end{equation*}
where the denominator can be arbitrary small, so $\nabla f_\alpha(x)$ is unbounded.
On the other hand, the Hessian
\begin{equation*}
    \nabla^2 f_\alpha(x)=-\mathbb{E}_p\frac{}{\langle p^\alpha, x^{1-\alpha}\rangle^2}
\end{equation*}
